# Supplementary material for: Attribute-Based Robotic Grasping with Data-Efficient Adaptation
Source: arXiv:2501.02149 source file (2025-01-04)
Supplement: Supplementary file 1 [file appendix_new.pdf]

## *A. Real-World Objects*

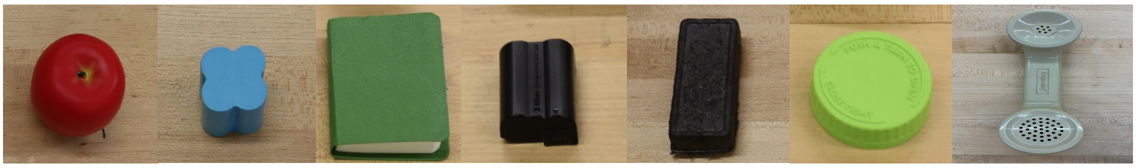

| Apple | Clover | Book | Battery | Eraser | Lid | PhoneHandler |
|---|---|---|---|---|---|---|
| red sphere | Blue cylinder | green cuboid | black cube | black cuboid | green cylinder | Yellow cuboid |

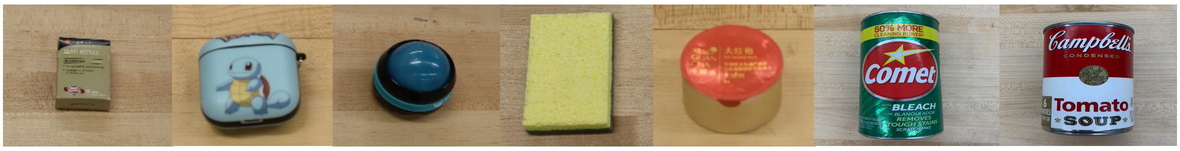


| LeadBox | PokemonCase | Roller | Sponge | TeaCan | CometBleach | TomatoCan |
|---|---|---|---|---|---|---|
| yellow cube | blue cube | blue sphere | yellow cuboid | red cylinder | green red cylinder | Red black cylinder |

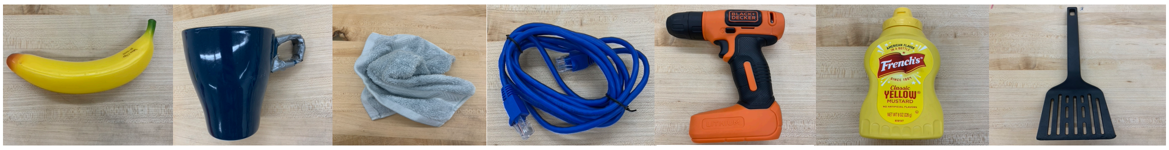


| Banana | BlueCup | BlueTowel | Cable | Drill | MustardBottle | Spatula |
|---|---|---|---|---|---|---|
| yellow | blue black cylinder | blue | blue | red black | yellow cuboid | black |

## *B. Simulated Novel Objects*

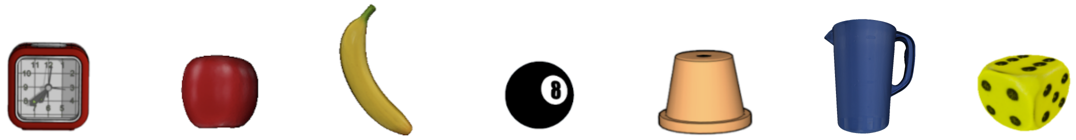

| AlarmClock | Apple | Banana | BilliardBall | BloemPot | BluePitcher | Dice |
|---|---|---|---|---|---|---|
| red cube | red sphere | yellow | black sphere | yellow cylinder | blue cylinder | yellow cube |

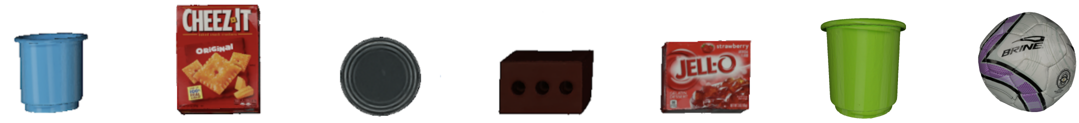


| Cup | CrackerBox | FishCan | FoamBrick | GelatinBox | GreenCup | Soccer |
|---|---|---|---|---|---|---|
| blue cylinder | red cuboid | black cylinder | red black cuboid | red cube | green cylinder | sphere |

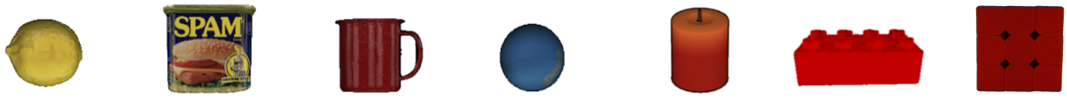


| Lemon | MeatCan | Mug | RacquetBall | Candle | RedLego | Rubicscube |
|---|---|---|---|---|---|---|
| yellow sphere | blue yellow cube | red cylinder | blue sphere | red cylinder | red cuboid | red blue cube |

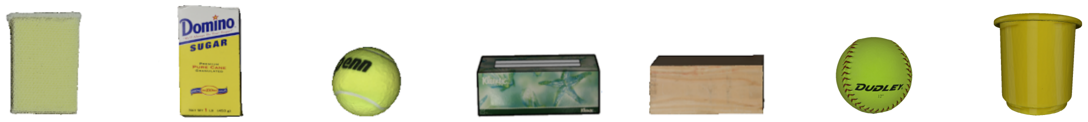

| Sponge | SugarBox | TennisBall | TissueBox | WoodBlock | SoftBall | YellowCup |
|---|---|---|---|---|---|---|
| yellow cuboid | yellow cuboid | green yellow sphere | green cuboid | cuboid | green sphere | yellow cylinder |

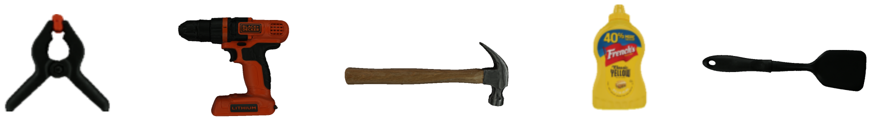

| Clamp | Drill | Hammer | MustardBottle | Spatula | YellowLego |
|---|---|---|---|---|---|
| black | red black | black | yellow blue cuboid | black | yellow cuboid |
