# Supplementary material for: Attribute-Based Robotic Grasping with Data-Efficient Adaptation
Source: arXiv:2501.02149 source file (2025-01-04)
Supplement: Supplementary file 2 [file 6appendix.tex]

\section{APPENDIX} \label{append}
\includepdf[pages={1}, offset=0 -0.6cm]{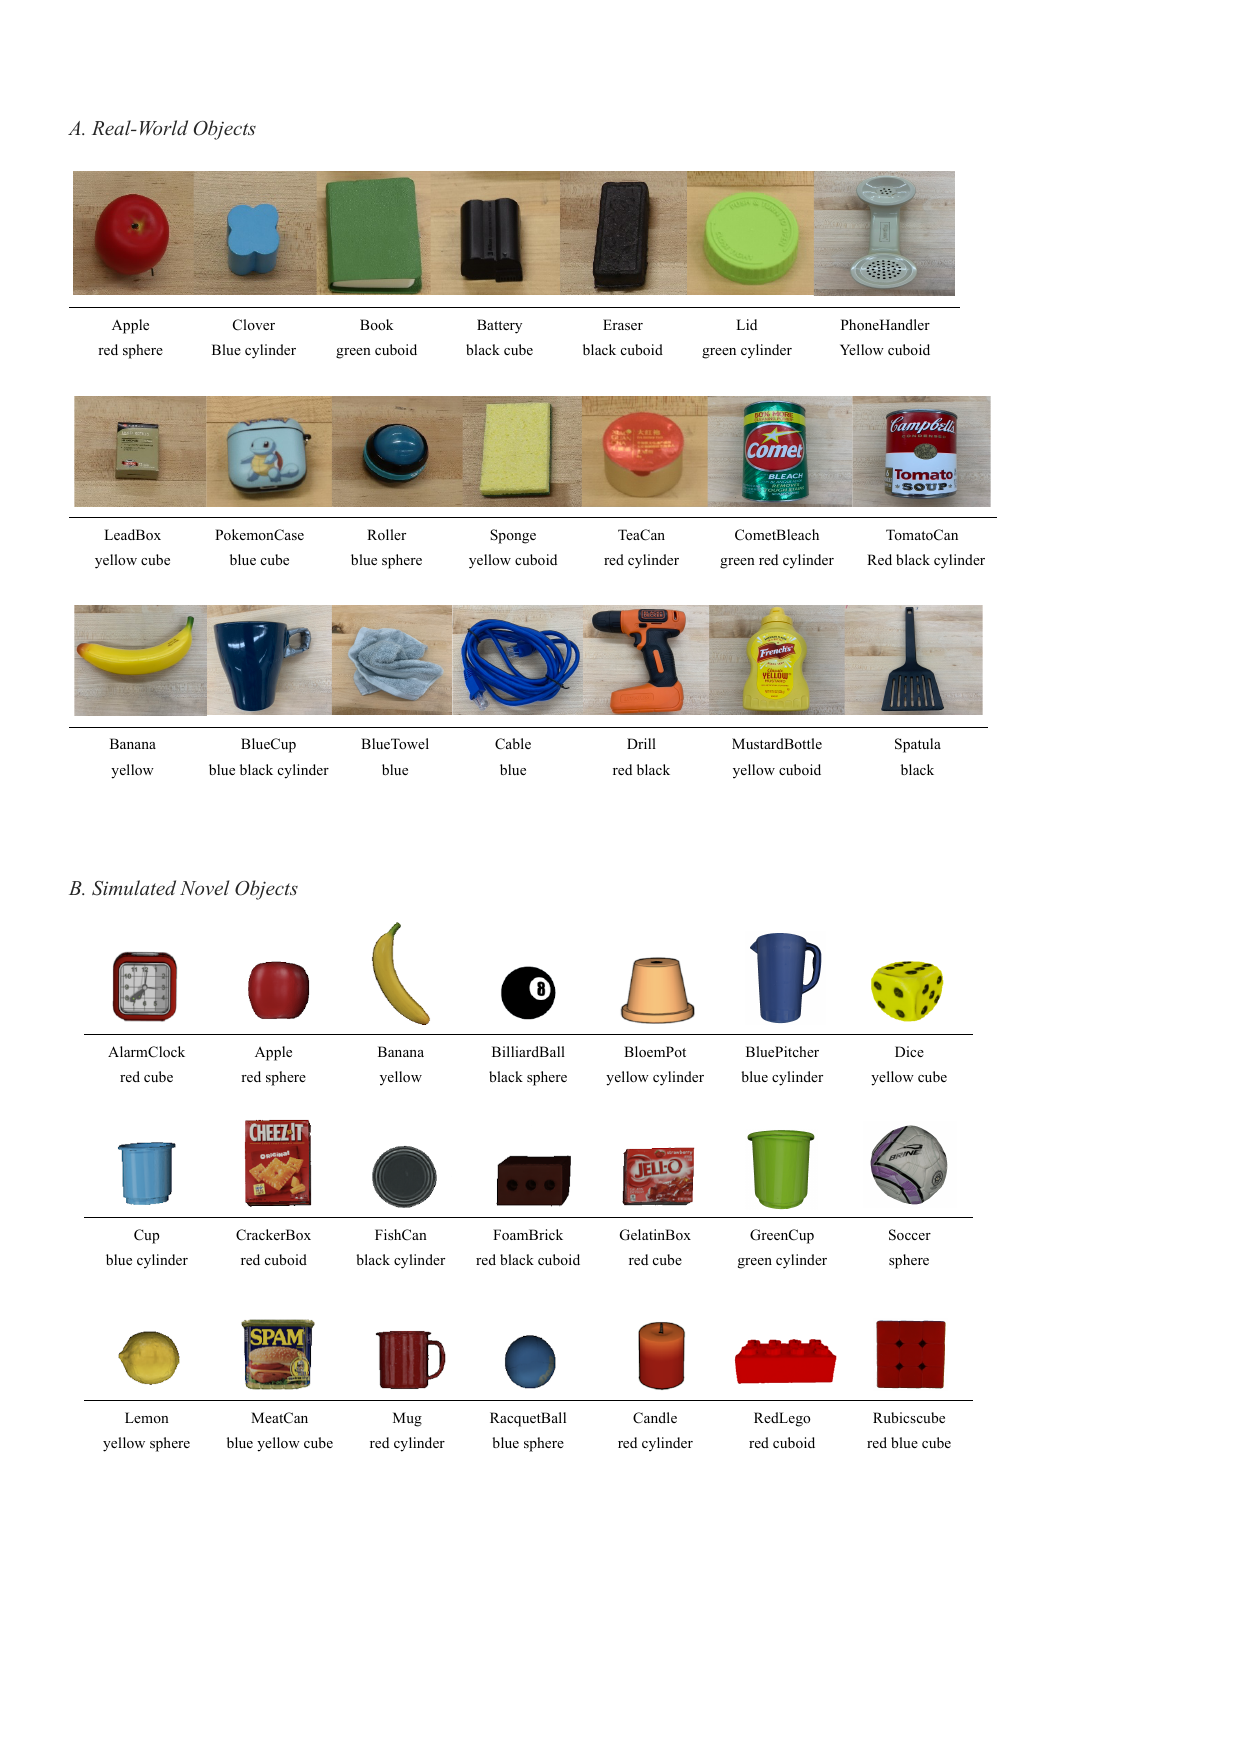}
\includepdf[pages={2}]{sections/appendix_new.pdf}
